# Supplementary material for: From Pixels to Feelings: Aligning MLLMs with Human Cognitive Perception of Images
Source: arXiv:2511.22805 source file (2025-11-27)
Supplement: Supplementary file 1 [file prompt1.pdf]

## Prompt for rewriting “from user” instruction:

You will see a visual-analysis instruction.
Rewrite it in fresh language **for the same sub-task** (Aesthetics).
• Important: Keep the **<image>** tag.
• Add brief explanation for this specific sub-task (Aesthetics) to the instruction.
• And also (in this specific order):
  • Ask the model to give a description label for the corresponding image, then
  • Ask the model to predict the scores based on this scores-label rules:

{
*- (0.0, 3.5, 'very low')*
*- (3.5, 5.0, 'low')*
*- (5.0, 6.5, 'medium')*
*- (6.5, 8.0, 'high')*
*- (8.0, 10.1, 'very high')*
}.

• Describe the scores prediction rule (e.g. exact three digits) after asking the model to return the label and the scores number.
• Ask the model to return only the label and the scores number, nothing else.

ORIGINAL:
<image> You are an expert in visual aesthetics. Please analyze the aesthetic value of the following image and assign a score from 1.000 to 10.000, using exactly three decimal places. The score should reflect nuanced judgment — not just whole or half values. Be precise and consider subtle details. Avoid defaulting to scores ending in .000 or .500 unless genuinely appropriate. Please only return a number without other comment

**Prompt for rewriting “from MLLM” (GT):**

A dataset stores only the numeric score **{5.241}** for the sub-task {Aesthetics}.
Rewrite that answer by:
• keeping the SAME numeric value
• Augment the answer with a short natural-language qualifier according to the label rules:
{
*- (0.0, 3.5, 'very low')*
*- (3.5, 5.0, 'low')*
*- (5.0, 6.5, 'medium')*
*- (6.5, 8.0, 'high')*
*- (8.0, 10.1, 'very high')*
}
• Returning only ONE line with the numeric score and the qualifier, nothing else.

ORIGINAL ANSWER:
**{5.241}**

Prompt for generating Qwen-Image T2I prompts:

- **Aesthetics**: describe something that require understanding of beauty, whether it's people or nature or plants.
- **Funniness**, require humorous cognition, know what is dramatic/funny.
- **Emotional**, can capture the emotion of a certain scene/facial expression.
- **Memorability**, describe a scene which will challenge the model to generate one that is more memorable (may give some details/vague description) and make the prompt a bit vague (but not too much) so it can test whether they have good understanding of the cognition.
- **General**, give general text-to-image generation prompts that test the quality of the generated images.
